# Supplementary material for: LLMs are Biased Teachers: Evaluating LLM Bias in Personalized Education
Source: arXiv:2410.14012 source file (2025-02-09)
Supplement: Supplementary file 1 [file app_generated.tex]

\section{Generated Text Examples}
\label{app:generated}
